# Supplementary material for: Quantifying Arbitrage in Automated Market Makers: An Empirical Study of Ethereum ZK Rollups
Source: arXiv:2403.16083 source file (2024-06-26)
Supplement: Supplementary file 1 [file 98AppendixFigures.tex]

\section{Additional Figures} \label{app:fig}

\begin{comment}
\begin{figure*}[ht]
  \centering
  \begin{minipage}[c]{0.5\textwidth}
    \centering
    \includegraphics[width=1\linewidth]{figures/SyncSwapETHBTC.png}
  \end{minipage}\hfill
  \begin{minipage}[c]{0.5\textwidth}
    \centering
    \includegraphics[width=1\linewidth]{figures/SyncSwapUSDCETH.png}
  \end{minipage} 

  \begin{minipage}[c]{0.5\textwidth}
    \centering
    \includegraphics[width=1\linewidth]{figures/zkSwapETHBTC.png}
  \end{minipage}\hfill
  \begin{minipage}[c]{0.5\textwidth}
    \centering
    \includegraphics[width=1\linewidth]{figures/zkSwapUSDCETH.png}
  \end{minipage}
  \caption{MAV for USDC-ETH pools and ETH-BTC at zkSwap and SyncSwap. It is good to see that Sync pool much more liquid and much more MAV too. Indeed, this makes sense since more trading needed to actually have a market impact from arbitrageurs. \DM{Need to be sure that max abs delta price shown and that MAV summed over misalignment periods and not all persistent cases.}} 
  \label{fig:MAVcharts}
\end{figure*}

\end{comment}
