# Supplementary material for: Quantifying Arbitrage in Automated Market Makers: An Empirical Study of Ethereum ZK Rollups
Source: arXiv:2403.16083 source file (2024-06-26)
Supplement: Supplementary file 2 [file 99Appendix.tex]

\section{Additional Information} \label{app:1}

(Debbie's Comment)

\section{Abb.}

 Test~\cite{Gogol2023SoK:Risks}.

\REVIEW{Example of a REVIEW.}

\PENDING{Example of a PENDING.}

\TODO{Example of a TODO.}

\MISSING{Example of a MISSING.}

\REVISIT{Example of a REVIST.}

\FIXME{Example of a FIXME.}{TEXT}

\REMOVE{Example of a REMOVE.}
